# Supplementary material for: Computing and Exploiting Document Structure to Improve Unsupervised Extractive Summarization of Legal Case Decisions
Source: arXiv:2211.03229 source file (2022-11-06)
Supplement: Supplementary file 1 [file Appendix_document_examples.tex]

% \section{Examples of Dataset}
% \subsection{CanLII Dataset}
% We include one example of the CanLII dataset with both case and summary. The IRC sentences are highlighted with the corresponding colors.
% \begin{table*}
% \begin{tabular}{c|c}
%      J. 2003 SKQB 487 D.I.V. A.D. 2003 No. 172 J.C. R. IN THE QUEEN’S BENCH (FAMILY LAW DIVISION) JUDICIAL CENTRE OF REGINA BETWEEN: CHRISTINE JAMES and RYAN MATTHEW ROSS (ROLLHEISER) RESPONDENT Jeffrey P. Reimer for the petitioner Donald G. Findlay for the respondent JUDGMENT DAWSON J. November 19, 2003 [1] At issue on this application is the interim custody of Keanna Marie James (Ross), child of the petitioner Christine James and the respondent Ryan Ross (Rollheiser) and, child support. INTERIM CUSTODY BACKGROUND FACTS [2] By way of background, the parties began to cohabit in May of 1998. In May of 1999, Keanna was born. Although there is conflicting affidavit evidence with regard to the date the parties ceased to cohabit, it is somewhere in the period between October of 1999 and April of 2000. Since the time the parties ceased to cohabit, Keanna has resided with the petitioner. The respondent has had access. [3] The respondent states in his affidavit dated October 3, 2003, that the parties had an arrangement in May and June of 2000, where the parties would “switch Keanna back and forth every second day,” and that after that the respondent had access to Keanna every weekend until November 2002 when, the respondent alleges, the petitioner ended access. The respondent says that in February 2003, the respondent was “allowed to have Keanna every second weekend, except for period of two weeks in March.” [4] The petitioner denies in her reply affidavit dated October 8, 2002, that the parties had any arrangement switching Keanna every second day or every weekend. She states that the parties had an arrangement from the outset whereby the respondent would see Keanna every second weekend and that is what happened. The petitioner asserts that the every second weekend access was interrupted over the years “by couple of violent episodes instigated by Ryan.” Counsel for the petitioner argued in chambers that the respondent made no attempts at gaining custody until he was served with the application of the petitioner. [5] have also reviewed the various affidavits of some of the family members and relatives of the parties. Although they are of no assistance in assisting me in determining the specific time periods wherein the respondent purported to have access to the child, they are nevertheless all consistent in establishing one thing; that the respondent did, in fact, have plenty of access to the child at various times from 1999 to 2003. [6] The petitioner herself, in her affidavit dated September 2, 2003, admits that since the parties ceased to cohabit, the respondent has “exercised access with their daughter on fairly regular basis.” As well, in her subsequent affidavit dated October 8, 2003, the petitioner confirms various access arrangements that the parties had, save for those she explicitly disputes. [7] The surplus of the various affidavits of the parties to the applications consist of accusations and constant strife about past access arrangements. The affidavits of the parties and their family members and relatives satisfy me that both parties are loving parents to their child. will also say that the mutual love and acceptance demonstrated by the families and relatives of each party, along with the overall concern for the best interests of the child, is self-evident and commendable. INTERIM CUSTODY LAW AND ANALYSIS [8] The purpose of an interim custody order is to give person the right and duty to care for child until permanent order or another interim order is made. On an interim application, the focus differs from that of permanent custody hearing. Rather than focussing on the long-term best interests of the child, court focusses on the short-term needs of the child. As a result, interim orders usually reinforce the status quo in an attempt to reflect on the best interests of the child. [9] Sections and of The Children’s Law Act, 1997, S.S. 1997, c. C-8.2 prescribe the relevant considerations in determining interim custody: 6(1) Notwithstanding sections to 5, on the application of parent or other person having, in the opinion of the court, sufficient interest, the court may, by order: (a) grant custody of or access to child to one or more persons; (b) determine any aspect of the incidents of the right to custody or access; and (c) make any additional order that the court considers necessary and proper in the circumstances. (2) Where the court grants custody of child to parent pursuant to subsection (1), the court, where in its opinion it would be in the best interests of the child to do so, may by order, authorize the parent to appoint person: (a) to have custody of the child on the parent’s death; (b) to be the guardian of the property of the child on the parent’s death; or (c) to have both of the duties mentioned in clauses (a) and (b). (3) On an application and prior to making an order pursuant to subsection (1), the court may make or vary an interim order on any terms and conditions it considers appropriate. ... In making, varying or rescinding an order for custody of child, the court shall: (a) have regard only for the best interests of the child and for that purpose shall take into account: (i) the quality of the relationship that the child has with the person who is seeking custody and any other person who may have close connection with the child; (ii) the personality, character and emotional needs of the child; (iii) the physical, psychological, social and economic needs of the child; (iv) the capacity of the person who is seeking custody to act as legal custodian of the child; (v) the home environment proposed to be provided for the child; (vi) the plans that the person who is seeking custody has for the future of the child; and (vii) the wishes of the child, to the extent the court considers appropriate, having regard to the age and maturity of the child; (b) not take into consideration the past conduct of any person unless the conduct is relevant to the ability of that person to act as parent of child; and (c) make no presumption and draw no inference as between parents that one parent should be preferred over the other on the basis of the person’s status as father or mother. [10] In considering an interim application the following questions might be posed, as noted by James G. McLeod in his book, Child Custody, Law Practice, 3d ed. (Toronto: Thomson Canada Limited, 1992, looseleaf, updated 2003): (a) Where and with whom is the child residing at the time of the interim hearing? (b) Where and with whom had the child been residing in the immediate past? (c) If there has been change in the child’s residence or primary caregiver in the recent past, why was the change made and who participated in the decision? (d) Are the child’s current living arrangements suitable for the child, taking into consideration the short-term needs of the child and the temporary nature of the order? (e) Is the current caregiver suitable role model and able to meet the child’s needs? (f) Are there any problems with the child’s current parenting or living arrangements? (g) Is there any reason to change the child’s current parenting or living arrangements? [11] Here I must take into account the current status quo, namely, that the child has and does reside with the petitioner, with access and visitation arrangements to the respondent. Keanna is doing well and has loving, stable relationship with her mother. The petitioner has provided suitable care and has met Keanna’s needs. Notwithstanding the instances of suspended access, the arrangements for access appear to have worked relatively well and appear to be in Keanna’s best interests. There is plenty of affidavit evidence to support this: (a) The petitioner admits that “in general, Ryan loves Keanna” and has exercised access to her on fairly regular basis; (b) Both parties have been willing to make arrangements in the past; (c) Efforts have been made by the respondent at contact with the child. (d) Efforts have been made by the respondent to make the child feel comfortable, happy while at his home; (e) Efforts have been made by the family members and relatives of both families to provide living environment for the child; and (f) Evidence that the child expresses content and joy with the respondent and his family (including new sister). [12] The respondent wishes to change the status quo on an interim basis to have Keanna reside with him every second week. The respondent has stated in an affidavit that he maintains odd work hours and suggests that if he had equal time with his daughter, his present wife would care for Keanna rather than having Keanna go to daycare as she presently does. This would be significant change in the status quo and one that is not yet established to be in Keanna’s best interests. [13] Based on the evidence before me, I make an order for interim custody to the petitioner with access to the respondent. The order is consistent with previous decisions of this Court. See for example Green v. Anderson, [1996] S.J. No. 752 (QL) (Q.B.), Kwok v. MacDonald, [1997] S.J. No. 478 (QL) (Q.B.), Hudson v. Hudson, 2000 SKQB 192 (CanLII); (2000), 192 Sask. R. 274 (Q.B.), Yurchak v. Yurchak, 2000 SKQB 213 (CanLII); (2000), 192 Sask. R. 312 (Q.B.), Prettyshield-Nicholls v. Maloughney, 2002 SKQB 299 (CanLII); [2002] S.J. No. 440 (QL) (Q.B.), and G.J.S. v. L.J.M., 2002 SKQB 417 (CanLII); [2002] S.J. No. 610 (QL) (Q.B.). [14] Both parents were ordered to complete the Parenting After Separation course. Both parties must file certificate of completion once the course is completed. [15] The parties raised in their material the issue of each other’s lack of cooperation and communication. While am not in position, at this stage, to decide whether or not the accusations of each party are substantiated, can say, with relative certainty, that there is an unhealthy degree of constant bickering. Keanna is likely affected to varying degrees by the discord between the parties. would go on to comment that it is evident that as long as the parties work on establishing better communication, the child will benefit from contact with both parents, with minimal disruption. [16] Accordingly, there will be the following order: (a) The petitioner shall have interim custody of Keanna Ross (James); (b) The respondent shall have reasonable access including every second weekend, reasonable telephone access and reasonable access during holiday periods. INTERIM CHILD SUPPORT [17] The respondent, on October 15, 2003, was ordered to file year to date income information. That has now been filed. find the respondent’s income for the purposes of interim child support to be $23,175.00. The respondent shall pay interim child support in the amount of $193.00 per month commencing on December 1, 2003 and a like amount on the first day of each month thereafter until further order. [18] find the petitioner’s income for the purposes of interim child support to be $4,921.96 (the average of her 2000 and 2001 income). [19] find the child care costs to be $125.00 per month. The respondent shall pay his proportionate share of childcare costs (being 82.5\%) in the amount of $103.00 per month commencing with $206.00 payable forthwith for October and November, 2003 and like amount on the first day of each month thereafter until further order. [20] The petitioner shall have costs of her application." & "At issue was the interim custody of the child and child support. HELD: Interim custody was given to the petitioner with access to the respondent. The respondent was ordered to pay interim child support in the amount of \$193 per month. On an interim custody application, the Court must take into account the status quo. \\

     
% \end{tabular}
% \caption{CanLII dataset}
% \end{table*}
